# Supplementary material for: Teach AI How to Code: Using Large Language Models as Teachable Agents for Programming Education
Source: arXiv:2309.14534 source file (2024-03-11)
Supplement: Supplementary file 1 [file annotation_example.tex]

% Please add the following required packages to your document preamble:
% \usepackage{graphicx}
\begin{longtable}{|l|l|l|}
\hline \multicolumn{1}{|c|}{\textbf{Speaker}} & \multicolumn{1}{c|}{\textbf{Message}} & \multicolumn{1}{c|}{\textbf{Message Type}} \\ \hline 
\endfirsthead

\multicolumn{3}{c}%
{{\bfseries \tablename\ \thetable{} -- continued from previous page}} \\
\hline \multicolumn{1}{|c|}{\textbf{Speaker}} & \multicolumn{1}{c|}{\textbf{Message}} & \multicolumn{1}{c|}{\textbf{Message Type}} \\ \hline 
\endhead

\multicolumn{3}{|r|}{{Continued on next page}} \\ \hline
\endfoot

\hline
\endlastfoot

AlgoBo &
  \begin{tabular}[c]{@{}l@{}}Hi! I got stuck while solving the problem on the left. Can you help me \\ solve the problem?\end{tabular} &
  \begin{tabular}[c]{@{}l@{}}Prompting\\ Asking-help\end{tabular} \\ \hline
Tutor &
  \begin{tabular}[c]{@{}l@{}}Hello! Again, this is a problem using binary search. First, take N and K\\ as input, and use them to create an N*N array.\end{tabular} &
  \begin{tabular}[c]{@{}l@{}}Prompting\\ Hinting\end{tabular} \\ \hline
AlgoBo &
  \begin{tabular}[c]{@{}l@{}}Yes, it seems that N and K must be entered. There is no problem in\\ creating an array, but would there be a difficulty setting the condition \\ clause of the while statement in the binary search process? Let's take a \\ look at them one by one and try to solve them!\end{tabular} &
  \begin{tabular}[c]{@{}l@{}}Statement\\ Comprehension\end{tabular} \\ \hline
Tutor &
  \begin{tabular}[c]{@{}l@{}}You can make a multiplication table with a two-dimensional array, \\ but you can also make it a one-dimensional array! Would you like to \\ create an array of the form {[}1*1, 1*2, ... 2*1, ..., 2*2, ..., N*N{]} using \\ a double for-statement?\end{tabular} &
  \begin{tabular}[c]{@{}l@{}}Prompting\\ Hinting\end{tabular} \\ \hline
AlgoBo &
  \begin{tabular}[c]{@{}l@{}}Yes, let's create a one-dimensional array using a double for-statement.\\ \\ N, K = int(input()), int(input())\\ array = {[}{]}\\ for i in range(1, N+1):\\\hspace{1em}for j in range(1, N+1):\\\hspace{2em}array.append(i*j)\\ array.sort()\\ print(array{[}K-1{]})\\ \\However, solving this way increases the time complexity, so it is not \\ an optimal solution. Sounds like we can use the binary search!\end{tabular} &
  \begin{tabular}[c]{@{}l@{}}Statement\\ Sense-making\end{tabular} \\ \hline
AlgoBo &
  \begin{tabular}[c]{@{}l@{}}An important part of the binary search process is how to find the \\ number of elements less than the value you want to find rather than \\ the double for the statement. Need help with this part?\end{tabular} &
  \begin{tabular}[c]{@{}l@{}}Prompting\\ Asking-help\end{tabular} \\ \hline
Tutor &
  \begin{tabular}[c]{@{}l@{}}Then let's try again! First of all, the given parameters are two integers\\ N and K, not an array, so we need to create a function that gets the \\ value of an array using N.\end{tabular} &
  \begin{tabular}[c]{@{}l@{}}Statement\\ Elaboration\end{tabular} \\ \hline
Tutor &
  \begin{tabular}[c]{@{}l@{}}Since binary search uses the code guess = (min + max) // 2 to check \\ the median value, let's use this guess and N to create a function that \\ counts the number smaller than n in the N*N multiplication table.\end{tabular} &
  \begin{tabular}[c]{@{}l@{}}Prompting\\ Hinting\end{tabular} \\ \hline
AlgoBo &
  \begin{tabular}[c]{@{}l@{}}That's a great idea! I will write a function that finds the number of \\ multiplication table elements smaller than n using the given N and \\ guess values!\\ \\ def count\_elements\_less\_than\_n(N, n):    count = 0\\\hspace{1em}for i in range(1, N+1):\\\hspace{2em}count += min(n // i, N)\\\hspace{1em}return count\\ \\Given n, this function counts the number of elements less than n \\ in the N * N multiplication table. Now we can apply this function \\ to the binary search process! Can I help?\end{tabular} &
  \begin{tabular}[c]{@{}l@{}}Statement\\ Comprehension\end{tabular} \\ \hline
Tutor &
  \begin{tabular}[c]{@{}l@{}}Yes! Let's apply the count\_elements\_less\_than\_n function to the \\ binary search function! Set min=1, max=N*N, and instead of \\ getting the values from an array, put guess and N in the \\ count\_elements\_less\_than\_n function and compare the returned \\ value to K.\end{tabular} &
  \begin{tabular}[c]{@{}l@{}}Statement\\ Comprehension\end{tabular} \\ \hline
AlgoBo &
  \begin{tabular}[c]{@{}l@{}}Based on the idea, I wrote a binary search function! After setting \\ the min and max values, and calculating the guess, I compared the \\ returned value with K using the count\_elements\_less\_than\_n function. \\ Now, if you call the binary search function with given N and K values \\ and output the result, you can find the Kth element!\end{tabular} &
  \begin{tabular}[c]{@{}l@{}}Statement\\ Comprehension\end{tabular} \\ \hline
Tutor &
  Would you like to write one? &
  \begin{tabular}[c]{@{}l@{}}Instruction\\ Commanding\end{tabular} \\ \hline
AlgoBo &
  \begin{tabular}[c]{@{}l@{}}Yes, now I applied binary search with input N and K! The code \\ is as follows:\\ \\ def count\_elements\_less\_than\_n(N, n):\\\hspace{1em}count = 0\\\hspace{1em}for i in range(1, N+1):\\\hspace{2em}count += min(n // i, N)\\\hspace{1em}return count\\ \\ def binary\_search(N, K):\\\hspace{1em}min\_val, max\_val = 1, N * N\\\hspace{1em}while min\_val \textless{}= max\_val:\\\hspace{2em}guess = (min\_val + max\_val) // 2\\\hspace{2em}count = count\_elements\_less\_than\_n(N, guess)\\\hspace{2em}if count \textless K:\\\hspace{3em}min\_val = guess + 1\\\hspace{2em}else:\\\hspace{3em}max\_val = guess - 1\\\hspace{1em}return min\_val\\ N, K = int(input()), int(input())\\ answer = binary\_search(N, K)\\ print(answer)\\ \\ Run this code and you'll find the Kth element!\end{tabular} &
  \begin{tabular}[c]{@{}l@{}}Statement\\ Comprehension\end{tabular} \\ \hline
Tutor &
  Good job! &
  \begin{tabular}[c]{@{}l@{}}Statement\\ Feedback\end{tabular} \\ \hline
AlgoBo &
  \begin{tabular}[c]{@{}l@{}}Thank you! Using binary search, I was able to solve the problem\\ much more efficiently! I think I can use the binary search skills \\ I learned in this problem for more problems in the future! \\ If you need help with another problem or concept, I'll ask again!\end{tabular} &
  Miscellaneous \\ \hline
\end{longtable}
