# Supplementary material for: Teach AI How to Code: Using Large Language Models as Teachable Agents for Programming Education
Source: arXiv:2309.14534 source file (2024-03-11)
Supplement: Supplementary file 2 [file mcq.tex]

\textbf{Merge Sort}

\begin{lstlisting}
How is the data set divided in the merge sort algorithm?

A) The data set is recursively divided into two equal (or nearly equal) halves until only individual elements remain.

B) The data set is divided into two parts based on a pivot element.

C) The data set is divided into sorted and unsorted parts.

D) The data set is divided into pairs of sequences.

A

Which of the following statements about merge sort is true?

A) Merge sort is a stable sort, maintaining the original order of the same elements.

B) Merge sort is an unstable sort, and the same elements may not maintain their original order.

C) Merge sort does not work well with linked lists.

D) Merge sort does not require a comparison function.

A

How does the merging process work in merge sort?

A) Merges the sub-arrays by directly inserting elements into the correct position in the original array.

B) Merges the sub-arrays by repeatedly selecting the smallest remaining element from the input sub-arrays.

C) Connects the sub-arrays by sorting each one and then merging.

D) Merges the sub-arrays by flipping the elements until they are in the correct order.

B

In the merge process of merge sort, what is the correct code to fill in the blank ___?

def merge(left, right):
    result = []
    while left and right:
        # ...
    result += ___
    return result

A) left + right

B) left * right

C) left - right

D) left / right

A

In the Python implementation of merge sort, to end the merging process, what condition should be checked?

def merge(left, right):
    result = []
    i = j = 0

    while ____:
        if left[i] < right[j]:
            result.append(left[i])
            i += 1
        else:
            result.append(right[j])
            j += 1

    result.extend(left[i:])
    result.extend(right[j:])
    return result

A) i < len(left) and j < len(right)

B) i >= len(left) or j >= len(right)

C) i > len(left) or j > len(right)

D) i < len(right) and j < len(left)

A

In the Python implementation of merge sort, to correctly merge the sorted halves of the list, what should replace ____?

def merge_sort(lst):
    if len(lst) <= 1:
        return lst

    mid = len(lst) // 2
    left = merge_sort(lst[:mid])
    right = merge_sort(lst[mid:])

    return ____

A) merge(left, right)

B) merge(lst[:mid], lst[mid:])

C) merge(mid)

D) merge(lst)

A

What is a noticeable advantage of merge sort over other comparison-based sorting algorithms such as quicksort or heapsort?

A) Merge sort does not require additional space.

B) Merge sort always operates in O(n log n) time, regardless of the initial order of the input.

C) Merge sort operates with a time complexity of O(n).

D) Merge sort is an in-place sorting algorithm.

B

While merge sort and quicksort are both divide-and-conquer algorithms, what is a noticeable difference in their operation?

A) Merge sort divides the array into two equal parts, while quicksort divides based on a pivot.

B) Quicksort divides the array into two equal parts, while merge sort divides based on a pivot.

C) Both algorithms divide the array in the same way.

D) Both algorithms either just merge or divide the array, they don't divide.

A

In which situation is the use of merge sort particularly effective?

A) When sorting an almost sorted array.

B) When sorting a small integer array.

C) When sorting a linked list.

D) When the order of identical elements doesn't matter.

C
\end{lstlisting}

\textbf{Breadth-first Search}

\begin{lstlisting}
\end{lstlisting}

\smallskip
\noindent
\textbf{Breadth-first Search}

\begin{lstlisting}
Which of the following descriptions about the characteristics of Breadth-First Search (BFS) is incorrect?

A) BFS starts from the root node and first visits adjacent nodes.

B) BFS uses less memory than Depth-First Search (DFS).

C) BFS uses a Queue data structure when visiting nodes.

D) BFS first visits the node that is farthest from the root node.

Answer: D

What data structure is typically used to record nodes visited during the Breadth-First Search (BFS) traversal of a graph?

A) Stack

B) Queue

C) Linked List

D) Binary Search Tree

Answer: B

Which traversal of a binary tree is the same as Breadth First Search (BFS)?

A) Pre-order Traversal

B) Post-order Traversal

C) Level-order Traversal

D) In-order Traversal

Answer: C

What data structure is typically used to record nodes visited during the Breadth-First Search (BFS) traversal of a graph?

A) Stack

B) Queue

C) Linked List

D) Binary Search Tree

Answer: B

Which traversal of a binary tree is the same as Breadth First Search (BFS)?

A) Pre-order Traversal

B) Post-order Traversal

C) Level-order Traversal

D) In-order Traversal

Answer: C

Below is a portion of Python code using BFS to find a path from the start node to the goal node in a graph. What is the most appropriate code for the blank?

```
if neighbour not in visited:
    visited.add(neighbour)
    queue.append(neighbour)
```

A) mid - 1

B) mid + 1

C) left - 1

D) right - 1

A

Below is a portion of Python code using BFS to traverse a graph. What is the most appropriate code for the blank?
```python
def binary_search(arr, x):
    low = 0
    high = len(arr) - 1
    mid = 0
 
    while low <= high:
        mid = (high + low) // 2
 
        ___
        else:
            return mid
 
    return -1
```
####
A)
```python
if arr[mid] < x:
    low = mid + 1
elif arr[mid] > x:
    high = mid - 1
```
##
B)
```python
if arr[mid] <= x:
    low = mid + 1
elif arr[mid] > x:
    high = mid - 1
```
##
C)
```python
if arr[mid] < x:
    low = mid
elif arr[mid] > x:
    high = mid
```
##
D)
```python
if arr[mid] > x:
    low = mid + 1
elif arr[mid] < x:
    high = mid - 1
```
####
A

Below is a portion of Python code using BFS to traverse a graph. What is the most appropriate code for the blank?

```python
def binary_search_recursive(arr, x, start, end):
    if ___:
        mid = (start + end) // 2
        if arr[mid] == x:
            return mid
        elif arr[mid] > x:
            return binary_search_recursive(arr, x, start, mid - 1)
        else:
            return binary_search_recursive(arr, x, mid + 1, end)
    return -1
```
####
A) start < end
##
B) start <= end
##
C) start === end
##
D) start > end
####
B


What is the main difference between Breadth-First Search (BFS) and Depth-First Search (DFS)?

A) BFS operates recursively, and DFS operates using a queue.

B) BFS uses a queue to visit nodes in order, and DFS uses a stack.

C) Both BFS and DFS use a stack.

D) Both BFS and DFS use a queue.

Answer: B

Which type of graph can't be traversed using BFS?

A) Cyclic graph

B) Acyclic graph

C) Connected graph

D) BFS can traverse all types of graphs.

Answer: D

Which is more efficient in searching for a value within a tree, BFS or Binary Search Tree (BST)?

A) BFS is more efficient than BST.

B) BFS and BST have the same efficiency.

C) BST is more efficient than BFS.

D) It depends on the type of graph.

Answer: C

\end{lstlisting}
